# Supplementary material for: Giant topological Hall effect in strained Fe$_{0.7}$Co$_{0.3}$Si epilayers
Source: arXiv:1312.1722 source file (2013-12-05)
Supplement: Supplementary file 1 [file TMS_THE_supp_submit.pdf]

# Giant topological Hall effect in strained $Fe_{0.7}Co_{0.3}Si$ epilayers
# **Supplementary Information**

Nicholas A. Porter, Priyasmita Sinha, Michael B. Ward, Alexey N. Dobrynin, Rik M. D. Brydson, Timothy R. Charlton, Christian J. Kinane, Michael D. Robertson, Sean Langridge, & Christopher H. Marrows

November 29, 2013

In this document we provide supplementary information on four topics: (i) we provide supporting evidence for the transmission electron microscope (TEM) analysis of our samples; (ii) we give additional information about the way in which our neutron reflectometry experiments were performed; (iii) we discuss our magnetotransport experiments including the way that we have tested for various possible artefacts; and (iv) we address the reason why the topological Hall effect does not cancel in our samples, which contain an equal mix of left- and right-handed chiral domains.

## S.1 Dark field TEM crystallography

Plan view TEM samples were aligned along the [111] zone axis (ZA) then tilted by 22° to the [321] ZA in order to determine the chiral structure of our films. We used a diffraction TEM technique along a different ZA to that previously used by Karhu *et al.*[1], and have recently become aware of an alternative convergent beam electron diffraction technique used to determine the structural chirality of thinned bulk crystals[2]. The selected area diffraction pattern obtained over multiple grains on the [321] ZA is shown in figure S1a. In order to accommodate the in-plane lattice mismatch between the Si substrate and the B20 epilayer, a 30° rotation around the [111] axis is required. The pattern in figure S1a comprises a superposition of the diffraction spots arising from a mixture left-handed and right-handed grains of $Fe_{0.7}Co_{0.3}Si$ aligned with $[11\bar{2}]$ $Fe_{0.7}Co_{0.3}Si$ $\parallel$ $[1\bar{1}0]$ Si and additional spots arising from double diffraction from $Fe_{0.7}Co_{0.3}Si$ grains of opposite chirality at the interfaces between the grains. A simulation of the superposition of left- and right-handed $Fe_{0.7}Co_{0.3}Si$ grains with such an alignment is shown in figure S1b showing good correspondence with the experimental diffraction spots from the film.

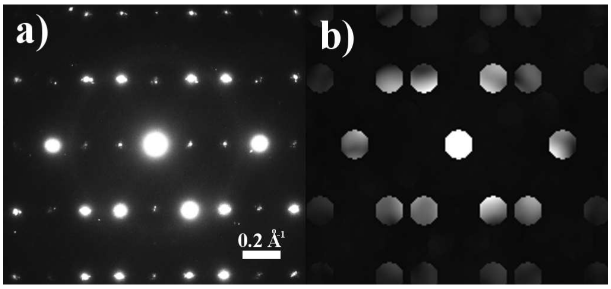


**Figure S1 | Plan-view TEM diffraction patterns of $Fe_{0.7}Co_{0.3}Si$ epilayer. a,** Diffraction pattern over multiple grains showing superposition of two aligned chiral grains viewed along the [321] ZA. **b,** Simulation of a superposition of aligned opposite handedness grains.

## S.2 Polarised Neutron Reflectometry

The film used for polarised neutron reflectometry (PNR), which we denote here FCS1, was grown separately to those used for all other measurements, which were taken from pieces of a single wafer called FCS2. Figure S2(a) shows the $\theta$-$2\theta$ X-ray diffraction (XRD) spectra. There is an excellent correspondence between the Bragg peaks from the two epilayers. Both the (111) and (222) peaks have a very similar full width at half maximum and intensity, with the peak positions corresponding to an interplanar spacing for FCS1 and FCS2 of $2.5721 \pm 0.0007$ Å and $2.5725 \pm 0.0007$ Å respectively, indistinguishable within the measurement uncertainty. The close match in lattice spacing is indicative of an almost identical stoichiometry for the two films[3,4] and the similarity in the peak shapes and intensity is indicative of a similar quality. Surface LEED patterns are shown in figure S2b demonstrating the good epitaxy obtained during growth for both films. Again both samples give very similar results and so we can expect that they will have directly comparable properties. Hence, we can expect that findings derived from PNR on FCS1 will be directly applicable to our understanding of the magnetotransport results derived from sample FCS2.

Low angle X-ray reflectometry (XRR) data for the sample used for PNR (FCS1) are shown in figure S3. There are clear Kiessig fringes indicating smooth and well-correlated top and bottom surfaces. The data have been fitted using the `GenX` software[5], with the fit shown as a solid line. The scattering length density (SLD) profile of this fitted model structure is is shown in the inset. It can be seen that a small 2 nm region of $\sim 10$ % higher density at the surface was required to produce a satisfactory fit to the data: otherwise the structure is just as expected from the nominal growth parameters. This near-surface region could be attributed to some oxidation which may or may not be magnetically inert.

PNR spectra for sample FCS1 are shown in figure S4. The data were acquired with a spin-polarised incident beam but without analysing the spin of the outgoing neutrons: hence only two neutron reflectivities are measured, denoted $R_+$ and $R_-$ for up and down neutron spins, respectively. The PNR data were corrected to account for the neutron polarisation and flipping efficiencies of the

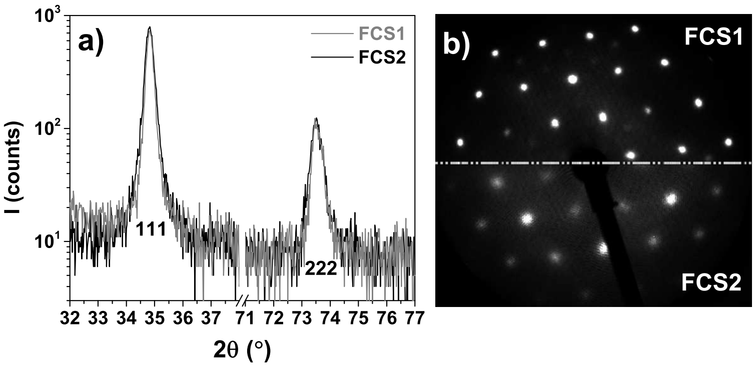


**Figure S2 | Crystallographic analysis of $Fe_{0.7}Co_{0.3}$Si epilayers. a,** High angle XRD of the two 50 nm $Fe_{0.7}Co_{0.3}$Si films used. FCS1 was used for PNR measurements, being 20 mm × 20 mm in shape, and FCS2 was divided and used for all other measurements. The samples are seen to be very similar. **b,** Low energy electron diffraction patterns from the two samples, again very similar.

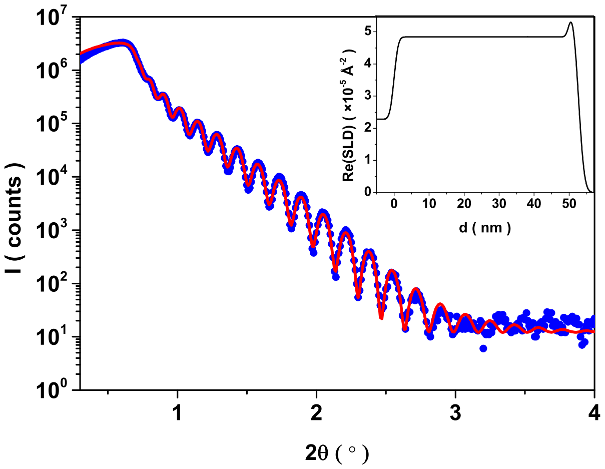


**Figure S3 | XRR of a 50 nm $Fe_{0.7}Co_{0.3}$Si epilayer, FCS1.** The solid line is a fit to the data (circles) provided by the scattering length density profile shown as an inset. This structural analysis was used to inform the fitting of the PNR data.

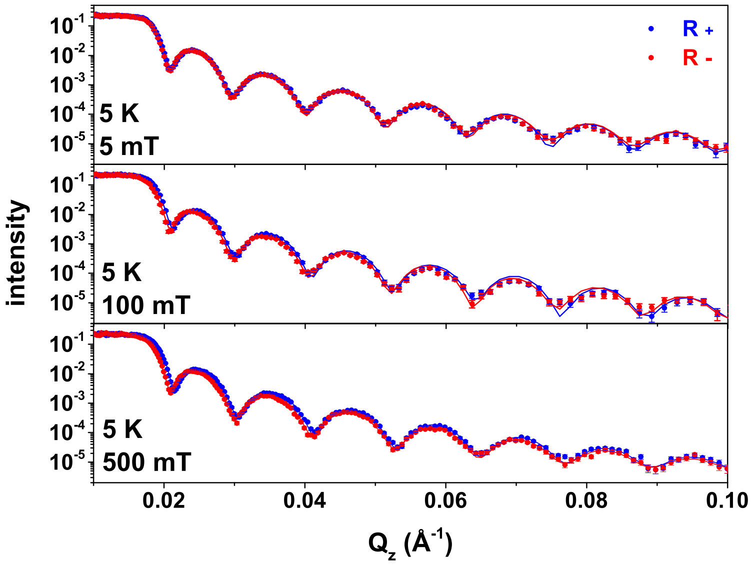


**Figure S4 | PNR of 50 nm $Fe_{0.7}Co_{0.3}Si$ film.** The solid lines are fits to the data (circles): blue data points are for spin-↑ neutrons, red data points are for spin-↓. The spin asymmetries arising from these data sets are shown in figure 3 of the main text.

POLREF beamline. We present data for three different thermomagnetic histories. In all three cases the sample was cooled from a temperature of $\sim$ 100 K, well above the magnetic ordering temperature, in a field of 5 mT, to 5 K. In the bottom plot, data taken after subsequently increasing the field to 500 mT at 5 K are shown. This field is large enough to magnetically saturate the sample, and a clear spin-splitting between the two neutron reflectivities is observed over the whole range of wavevector transfer $Q$. In the middle panel the measurement field applied at 5 K was 100 mT, and in the top panel the sample was simply held at 5 mT and measured. In these latter two cases the magnetisation is not saturated, and the spin-splitting is much reduced, particularly at low $Q$, and especially so in the 5 mT measurement. The spin asymmetries shown in figure 3 of the main article are derived from these data as the difference between the two curves normalised by their sum.

Again the `GenX` code was used to fit the data, with the fits shown as the solid lines in figure S4. The sample can be modelled successfully as a uniformly magnetised slab in the case of the 500 mT measurement field. The thickness is the same as that determined from XRR and the magnetisation is that expected for $Fe_{0.7}Co_{0.3}Si$, to within experimental error. The associated magnetic SLD is shown in figure 3 of the main article, along with the fits of the spin-asymmetry data that are presented there.

In the cases of the two measurements made at lower fields, it is clear that a uniformly magnetised slab is not the correct model: reduction of the magnetisation below the saturated value would lead to a reflectivity spectrum where the spin-asymmetry was reduced by the same factor at all values of $Q$. This

is seen not to be the case: the spin asymmetry is higher at large $Q$, with a marked feature just below $Q \approx 0.08$ Å$^{-1}$. In order to reproduce this feature, it is necessary to introduce a depth profile to the magnetic SLD. We have been able to successfully fit the data by assuming a spin-density wave constructed by adding together the left- and right-handed spin helices in the different chiral domains. This is reasonable since the lateral coherence length of the neutron beam is several microns, so that it reflects coherently from a large number of individual helical domains. The spins remain in the sample plane due to demagnetising and magnetocrystalline anisotropy effects, so that the propagation direction of the proper screw spin-helix is normal to the plane in our model. In both cases we obtain a periodicity of the magnetic profile of $\lambda_{\mathrm{epi}} = 9.3 \pm 0.5$ nm corresponding to a helical wavevector of $k_{\mathrm{epi}} = 2\pi/\lambda_{\mathrm{epi}} = 0.68 \pm 0.04$ nm$^{-1}$.

# S.3 Further details of magnetotransport measurements

## S.3.1 Experimental determination of the topological Hall effect contribution

Determination of the topological Hall contribution to $\rho_{xy}$ is done by making subtractions of other contributions from the measured total Hall resistivity. The ordinary Hall effect (OHE) contribution $\rho^{\mathrm{o}}_{xy}$ adds a linear contribution matching the slope in the high field regime where all other contributions are expected to be independent of the applied field $H$. Subtracting the anomalous Hall contribution (AHE) $\rho^{\mathrm{a}}_{xy} = R_{\mathrm{s}}M$ is non-trivial, since this contribution is hysteretic in $H$. We have implemented the method that has been used by a number of other groups for doing this[6–9], which is to use a measured conventional magnetometry hysteresis loop to determine the hysteretic form of $M(H)$.

The total Hall resistivity that is measured is given by

$$\rho_{xy} = \rho^{\mathrm{o}}_{xy} + \rho^{\mathrm{a}}_{xy} + \rho^{\mathrm{t}}_{xy}, \tag{S1}$$

where the ordinary Hall effect, $\rho^{\mathrm{o}}_{xy} = R_0 H$, is proportional to the applied field and $\rho^{\mathrm{t}}_{xy}$ is the topological contribution. The anomalous contribution has three components[9,10]:

$$\rho^{\mathrm{a}}_{xy} = \left[\alpha\rho_{xx0} + \beta\rho^2_{xx0} + b\rho^2_{xx}(H)\right] M(H). \tag{S2}$$

The terms with coefficients of $\alpha$, $\beta$, $b$ correspond to skew scattering, side-jump scattering and intrinsic contributions, respectively. As our films are doped semiconductors and have no residual resistivity, $\rho_{xx0}$, in the sense that it is usually measured, we approximate this by extrapolating the non-magnetic temperature dependence of the resistivity (above 70 K) to low temperatures, as shown in figure S5, thus neglecting additional magnetic contributions[11]. Manyala *et al.*[12] and Nagaosa *et al.*[10] conclude that skew scattering is a small contribution to the AHE for bulk $\mathrm{Fe}_{1-x}\mathrm{Co}_x\mathrm{Si}$, which we choose to neglect also. By measuring the out-of-plane longitudinal resistivity, $\rho_{xx}(H)$ and neglecting skew scattering, the AHE from equation S2 can be written as

$$\begin{aligned} \rho^{\mathrm{a}}_{xy} &= \beta\rho^2_{xx0}M(H) + b\rho^2_{xx}(H)M(H) \\ &\sim (\beta + b)\rho^2_{xx}(H)M(H) \sim S_{\mathrm{H}}\rho^2_{xx}(H)M(H). \end{aligned} \tag{S3}$$

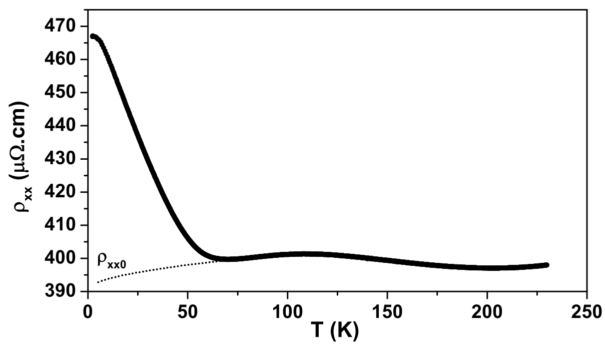


**Figure S5 | Estimating the residual resistivity.** The temperature dependence of the longitudinal resistivity was used to predict the residual resistivity $\rho_{xx0}$ neglecting the low temperature magnetic contribution to scattering below 70 K.

We found that $\rho_{xx0}^2 M(H)$ scaled with $\rho_{xx}(H)^2 M(H)$ to within 0.5 % over the whole field range used, and so the coefficients ($\beta$ and $b$) were consolidated into one coefficient $S_{\mathrm{H}}$. This scaling parameter and $R_0$ were then the only parameters used to fit the magnetisation, $M(H)$, to the total Hall effect, $\rho_{xy}$, as the scaled magnetisation, $\eta$, using

$$\eta = \rho_{xy}^{\mathrm{o}} + \rho_{xy}^{\mathrm{a}} \sim R_0 H + S_H \rho_{xx}^2(H) M(H). \tag{S4}$$

The THE was then obtained as the difference between $\rho_{xy}(H)$ and $\eta$. Figure S6a shows Hall resistivity $\rho_{xy}$ and scaled magnetisation $\eta$ measurements made at a variety of temperatures, from 5-100 K, for our $Fe_{0.7}Co_{0.3}Si$ Hall bar. At all temperatures it is possible to scale the high field (greater than $\sim$ 800 mT, see inset) magnetisation so that it matches the $\rho_{xy}$ very well. This indicates that we are properly capturing the anomalous Hall contribution to the measured total Hall resistivity. The differences between the pairs of curves are plotted in figure S6b, showing the temperature evolution of the topological Hall contribution $\rho_{xy}^{\mathrm{t}}$ to the Hall resistivity. These curves are selections from the set of isothermal field sweeps that were used to construct the phase diagram in figure 5 of the main text. As well as moving to lower values of magnetic field as $T$ rises, the THE peak also shrinks in magnitude.

### S.3.2 Temperature dependence of topological contributions to the resistivity tensor

The temperature dependence of $\rho_{xy}^{\mathrm{t}}$ is shown in figure S7, extracted as the peak value of that parameter (obtained at the sharp extremum) during each isothermal field sweep. The value declines montonically as the temperature is raised, vanishing at the ordering temperature. Since the THE does not arise from scattering, it should, in principle, not have any temperature dependence. However, since the magnitude of the THE signal is given by $\rho_{xy}^{\mathrm{t}} = -n_{\mathrm{s}} \Phi_0 P R_0$, any variation with temperature in any of these parameters will yield a temperature dependent THE signal. Whilst the magnetic flux quantum $\Phi_0 = h/e$ is a fundamental constant of nature, the spin-polarisation $P$, skyrmion winding

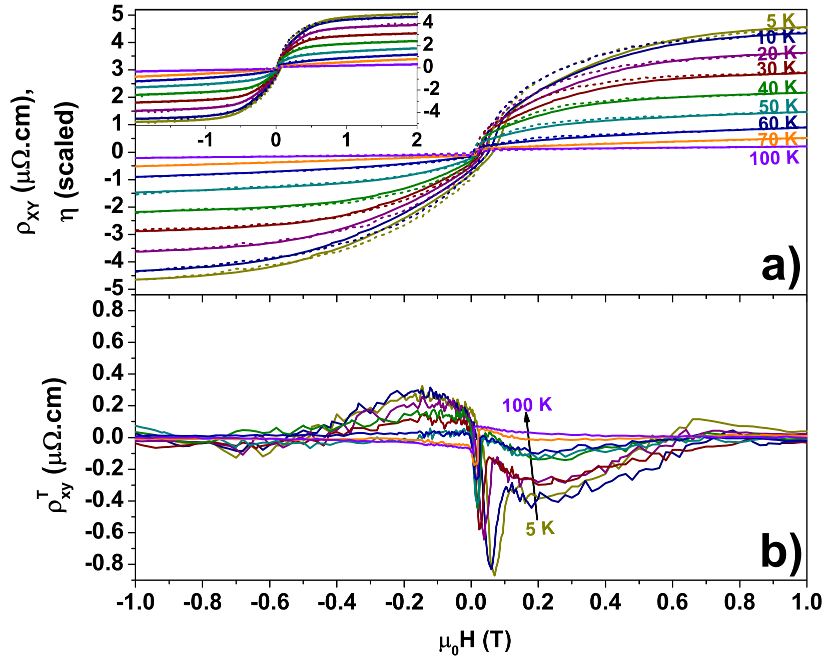


**Figure S6 | Determining the topological Hall contribution to $\rho_{xy}$.** **a,** Scaled magnetisation $\eta$ (dashed lines) and Hall resistivity $\rho_{xy}$ (solid lines) at selected temperatures. **b,** The difference between the isothermal data sets in **a** is plotted as a function of field, revealing the topological Hall contribution.

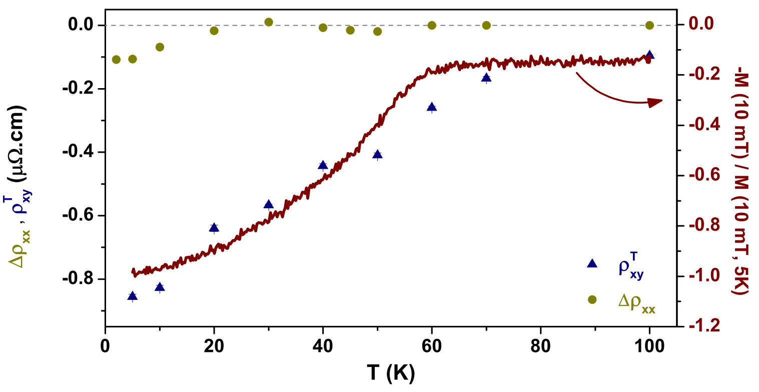


**Figure S7 | Temperature dependence of the topological parts of the Hall and longitudinal resistivities.** The extremum in the symmetric part of the field sweep in the out of plane geometry magnetoresistance ($\Delta\rho_{xx}$) is approximately an order of magnitude smaller than the extremum in the THE ($\rho^{\mathrm{t}}_{xy}$) and vanishes at a temperature of about 20 K, far below the ordering temperature of $T^{\mathrm{ord}}_{\mathrm{epi}} \approx 60$ K.

number density $n_{\mathrm{s}}$, and ordinary Hall constant $R_0$ are expected to be temperature dependent. Since $P$ is expected to be proportional to the magnetisation $M$, a scaled magnetisation curve $M(T)$ is also shown for comparison. This can be seen to yield the predominant contribution to the $T$ dependence of $\rho^{\mathrm{t}}_{xy}$. The small discrepancy near the ordering temperature can be attributed to changes to the other parameters, most probably the skyrmion density $n_{\mathrm{s}}$, in the near-critical regime.

In figure S7 we also show the equivalent temperature dependence for the residual (and possibly topological) contribution to the magnetoresistance $\Delta\rho_{xx}$. This is roughly one order of magnitude smaller at low temperatures, but also vanishes above a temperature of only about 20 K, well below the magnetic ordering transition. The origin of this much stronger temperature dependence is unknown. We speculate that it is related to the phase coherence of the electron wavefunctions.

## S.4 Absence of cancellation of the topological Hall effect

The fact that our sample is racemic, *i.e.* composed of roughly equal amounts of material with left- and right-handed crystal chiralities, implies that the chirality of the magnetism in these regions should also have opposite handedness, since the sign of the DMI vector $\mathbf{D}$ will be opposite[13]. When the skyrmion-like phase is entered, the in-plane vorticity of spins will therefore rotate in opposite directions in these regions. The out-of-plane magnetisation components will remain the same, as they are defined by the external field direction. One might naïvely expect that these two opposite in-plane chiralities will lead to opposing contributions to the topological Hall effect, and so the overall signal from our sample should be zero. Nevertheless, a large signal is in fact measured.

The spin Berry phase accumulated by an electron as it passes through a spin texture defined by $\mathbf{S}(\mathbf{r})$ is proportional to $\mathbf{S} \cdot (\partial_x \mathbf{S} \times \partial_y \mathbf{S})$ [14]. As a result the topological Hall resistivity is also proportional to this expression.

To see the independence of the THE on the in-plane spin direction winding direction, note that the two possible chiral configurations are related to each other simply by a shift of azimuthal angle, $\phi_{\circlearrowleft} = \phi_{\circlearrowright} + \pi$ (where $\phi_{\circlearrowleft}$ and $\phi_{\circlearrowright}$ are the angles in the $x$-$y$ plane for positive and negative in-plane chirality skyrmions, respectively, defined by $\phi = \arctan\left(S_x/S_y\right)$). Thus the Berry phase, which is proportional to $\sin\theta(\partial_x\theta\partial_y\phi - \partial_y\theta\partial_x\phi)$ in spherical co-ordinates, is the same in both cases, as it depends only on spatial derivative of $\phi$, and so is insensitive to the addition of a constant. This shows that domains with opposite in-plane windings will contribute additively to the overall topological Hall effect of the entire system, and so a racemic system such us ours should have a finite topological Hall effect.

# References


[1] Karhu, E. *et al.* Structure and magnetic properties of MnSi epitaxial thin films. *Phys. Rev. B* **82**, 184417 (2010).

[2] Morikawa, D., Shibata, K., Kanazawa, N., Yu, X. Z. & Tokura, Y. Crystal chirality and skyrmion helicity in MnSi and (Fe,Co)Si as determined by transmission electron microscopy. *Phys. Rev. B* **88**, 024408 (2013).

[3] Shinoda, D. Magnetic properties of $Co_{1-x}Fe_xSi$, $Co_{1-x}Mn_xSi$, and $Fe_{1-x}Mn_xSi$ solid solutions. *Phys. Stat. Solidi (a)* **11**, 129–135 (1972).

[4] Sinha, P., Porter, N. A. & Marrows, C. H. Strain-induced effects on the magnetic and electronic properties of epitaxial FeCoSi thin films (2013). arXiv:1307.7301 [cond-mat.mtrl-sci].

[5] Björck, M. & Andersson, G. GenX: an extensible X-ray reflectivity refinement program utilizing differential evolution. *J. Appl. Crystallogr.* **40**, 1174–1178 (2007).

[6] Lee, M., Onose, Y., Tokura, Y. & Ong, N. P. Hidden constant in the anomalous Hall effect of high-purity magnet MnSi. *Phys. Rev. B* **75**, 172403 (2007).

[7] Kanazawa, N. *et al.* Large topological Hall effect in a short-period helimagnet MnGe. *Phys. Rev. Lett.* **106**, 156603 (2011).

[8] Huang, S. X. & Chien, C. L. Extended skyrmion phase in epitaxial FeGe(111) thin films. *Phys. Rev. Lett.* **108**, 267201 (2012).

[9] Li, Y. *et al.* Robust formation of skyrmions and topological Hall effect anomaly in epitaxial thin films of MnSi. *Phys. Rev. Lett.* **110**, 117202 (2013).

[10] Nagaosa, N., Sinova, J., Onoda, S., MacDonald, A. H. & Ong, N. P. Anomalous Hall effect. *Rev. Mod. Phys.* **82**, 1539–1592 (2010).

[11] Onose, Y., Takeshita, N., Terakura, C., Takagi, H. & Tokura, Y. Doping dependence of transport properties in $Fe_{1-x}Co_xSi$. *Phys. Rev. B* **72**, 224431 (2005).

[12] Manyala, N. *et al.* Large anomalous Hall effect in a silicon-based magnetic semiconductor. *Nature Mater.* **3**, 255–262 (2004).

[13] Grigoriev, S. V. *et al.* Crystal handedness and spin helix chirality in $Fe_{1-x}Co_xSi$. *Phys. Rev. Lett.* **102**, 037204 (2009).

[14] Tatara, G., Kohno, H. & Shibata, J. Microscopic approach to current-driven domain wall dynamics. *Physics Reports* **468**, 213–301 (2008).
